# Supplementary material for: Curiosity as filling, compressing, and reconfiguring knowledge networks
Source: arXiv:2204.01182 ancillary file (2022-04-03)
Supplement: Supplementary file 1 [file Supplement.pdf]

# Supplement: Curiosity as filling, compressing, and reconfiguring knowledge networks

Shubhankar P. Patankar[a], Dale Zhou[b], Christopher W. Lynn[c,d], Jason Z. Kim[a], Mathieu Ouellet[e], Harang Ju[b], Perry Zurn[f], David M. Lydon-Staley[a,g,h], and Dani S. Bassett[a,e,i,j,k,l,*]

[a]Department of Bioengineering, School of Engineering and Applied Science, University of Pennsylvania, Philadelphia, PA 19104 USA
[b]Neuroscience Graduate Group, Perelman School of Medicine, University of Pennsylvania, PA 19104 USA
[c]Initiative for the Theoretical Sciences, Graduate Center, City University of New York, New York, NY 10016 USA
[d]Joseph Henry Laboratories of Physics, Princeton University, Princeton, NJ 08544 USA
[e]Department of Electrical and Systems Engineering, School of Engineering and Applied Science, University of Pennsylvania, Philadelphia, PA 19104 USA
[f]Department of Philosophy, American University, Washington, DC 20016 USA
[g]Annenberg School for Communication, University of Pennsylvania, Philadelphia, PA 19104 USA
[h]Leonard Davis Institute of Health Economics, University of Pennsylvania, Philadelphia, PA 19104 USA
[i]Department of Psychiatry, Perelman School of Medicine, University of Pennsylvania, Philadelphia, PA 19104 USA
[j]Department of Neurology, Perelman School of Medicine, University of Pennsylvania, Philadelphia, PA 19104 USA
[k]Department of Physics and Astronomy, College of Arts and Sciences, University of Pennsylvania, Philadelphia, PA 19104 USA
[l]Santa Fe Institute, Santa Fe, NM 87501 USA
[*]To whom correspondence should be addressed: dsb@seas.upenn.edu

April 3, 2022

# 1 Representations of knowledge

In building the reader's intuition for network representations of knowledge, we first motivate cognitive embeddings of conceptual knowledge with a summary of embeddings of physical spaces. In one view, internal representations of space take the form of cognitive maps that possess a metric Euclidean geometry [1]. The basis of such maps is spatially-tuned cells in the hippocampal-entorhinal system. In the hippocampus, specific place cells become active when individuals find themselves in specific environmental locations [2]. In the neighboring entorhinal cortex, grid cells [3]—named for their hexagonal lattice-like firing fields—integrate information about location [4], Euclidean distance [5], and goal direction [6, 7] to facilitate the rapid computation of vector paths between distant locations [8]. Evidence for grid cells was found in direct intracranial recordings of neural activity in pre-surgical epilepsy patients [9], and indirectly in functional magnetic resonance imaging (fMRI) data acquired from healthy individuals [7, 10]. During virtual spatial navigation tasks, in a phenomenon known as *hexadirectional modulation*, peaks in the macroscopic BOLD signal (acquired from fMRI) were observed for heading angles spaced 60° apart [7, 10]. This six-fold symmetry is a reflection of the hexagonal lattices formed by the firing fields of grid cells. Collectively, place and grid cells are constituents of the neural substrate that enables human navigation of continuous physical space.

Recent reports suggest that cognitive maps of conceptual knowledge share organizing principles with cognitive maps of physical space. Analogous to place cells that encode specific locations, concept cells in the medial temporal lobe encode specific concepts [11, 12]. For instance, one neuron was found to respond selectively to images of *The Beatles*, while another responded only to images of *The Simpsons* [11]. Moreover, hexadirectional modulation was observed when individuals interacted with a continuous two-dimensional space of birds of varying neck and leg lengths, implying the presence of a grid-like neural code for conceptual knowledge [13]. Related work has shown that participants learn map-like cognitive representations of a discrete two-dimensional social attribute space with axes for popularity and competence [14, 15]. Euclidean distances between individuals in the social hierarchy were linearly associated with hippocampal-entorhinal activity. In a social navigation task set up as a "create-your-own-adventure" computer game, interactions with people perceived as having more social influence induced greater changes in the hippocampal BOLD signal [16]. The same study found that activity levels in the posterior cingulate cortex were related to the Euclidean distance between individuals. Thus, evidence from a variety of continuous and discrete non-spatial domains supports the view that the brain organizes non-spatial knowledge into cognitive maps.

An alternative view conceptualizes internal representations as cognitive graphs rather than as Euclidean cognitive maps [17]. In a graph, discrete entities—such as locations in physical space or concepts in a conceptual space—are represented as nodes connected by edges. A key point of distinction between a purely map-based view and a purely graph-based view is the absence of a global coordinate system in the latter. As a result, distances between nodes are measured as relative topological path lengths. Some spatial navigation studies report violations of Euclidean rules such as symmetry and additivity, offering evidence against a purely map-based account [18]. Furthermore, a key affordance of cognitive maps is the ability to flexibly navigate between distant locations in physical space along previously unseen routes. Interestingly, though, humans can also successfully navigate non-Euclidean virtual environments in a similar manner [19, 20, 21]. The apparent conflict between the two accounts can be reconciled by viewing mental representations as labeled cognitive

graphs, where each node is accompanied by local (rather than global) metric information such as distances and angles to its immediate neighboring nodes [17, 18]. During a spatial navigation task, participants not only learned the graph structure of object locations in a maze but also showed a preference for traveling the shortest metric distances [22]. In our graph-based approach to curiosity, we build on labeled cognitive graphs to assume that distances between concepts can be computed not only as topological path lengths but also with a Euclidean metric [17].

## 2 Mechanical features of knowledge networks

In our network operationalization of the conformational change theory, we compute the embedding dimensionality and available conformational degrees of freedom for each growing knowledge network using Algorithm 1.

**Algorithm 1** Embedding dimensionality and available degrees of freedom for growing networks.

```
all_d ← [ ]
all_conformable_DoF ← [ ]
d ← 1                                                  ▷ initialize dimensionality to 1
for subgraph G_p ⊂ G do
    all_DoF ← d × nodes(G_p) − edges(G_p)
    rigid_DoF ← d × (d + 1)/2
    conformable_DoF ← DoF − rigid_DoF
    while conformable_DoF < 0 do     ▷ number of conformational motions cannot be negative
        d ← d + 1                                      ▷ increment dimensionality
        DoF ← d × nodes(G_p) − edges(G_p)
        rigid_DoF ← d × (d + 1)/2
    end while
    conformable_DoF ← DoF − rigid_DoF
    all_d.append(d)
    all_conformable_DoF.append(conformable_DoF)
end for
```

# 3 Generative network models

Generative models with simple growth rules can provide significant insight into whether network features of interest can distinguish structure from randomness. For instance, does the number of topological cavities increase with growth for *all* networks? Or might this be a consequence specific to growing knowledge networks? To answer questions such as these, we generate filtrations of toy networks with three distinct growth rules. For each model, we generate 100 networks with $N = 70$ nodes.

- The constant probability model: An edge is added between the $p$-th node in a filtration and all previous nodes with probability equal to 0.4. Therefore, the rank of a node has no impact on its likelihood of linking to previously added nodes.
- The proportional probability model: An edge is added between the $p$-th node in a filtration and all previous nodes with probability equal to $p/N$. Therefore, nodes added later in a filtration have a higher likelihood of being connected to previously added nodes.
- The preferential attachment model: Starting with a fully-connected skeleton of $m_0$ nodes, the $p$-th node in a filtration is connected to $m$ previously added nodes with a probability proportional to the degree of each node present. Since nodes with high degree continue to form more connections at the expense of low-degree nodes, this approach creates networks with heavy-tailed degree distributions. We set $m_0 = m = 4$.

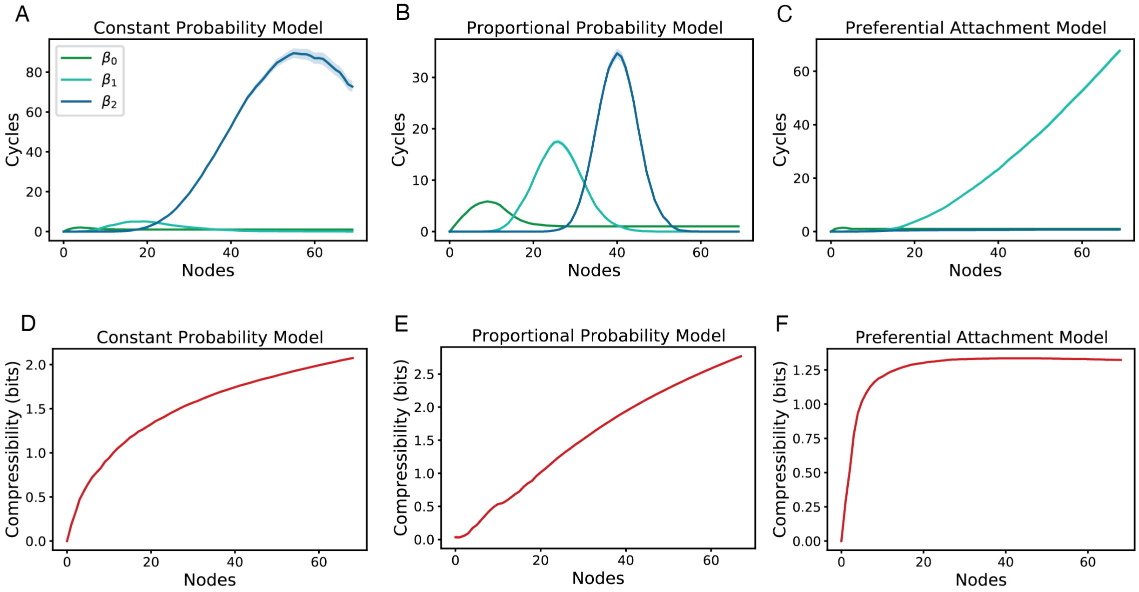


Figure 1: **Topological cavities and compressibility for generative network models.** Betti curves for the *(A)* constant probability, *(B)* proportional probability, and *(C)* preferential attachment models. Except for dimension 1 in the preferential attachment model, Betti numbers do not increase monotonically. The number of cycles typically first increases and then decreases as a function of network size. Compressibility curves for the *(D)* constant probability, *(E)* proportional probability, and *(F)* preferential attachment models. Compressibility increases monotonically for the constant and proportional probability models. The rate of increase appears to be higher for the constant probability model compared to the proportional probability model. In the preferential attachment model, the compressibility curve plateaus roughly upon the addition of the 20-th node. Shaded regions represent standard error.

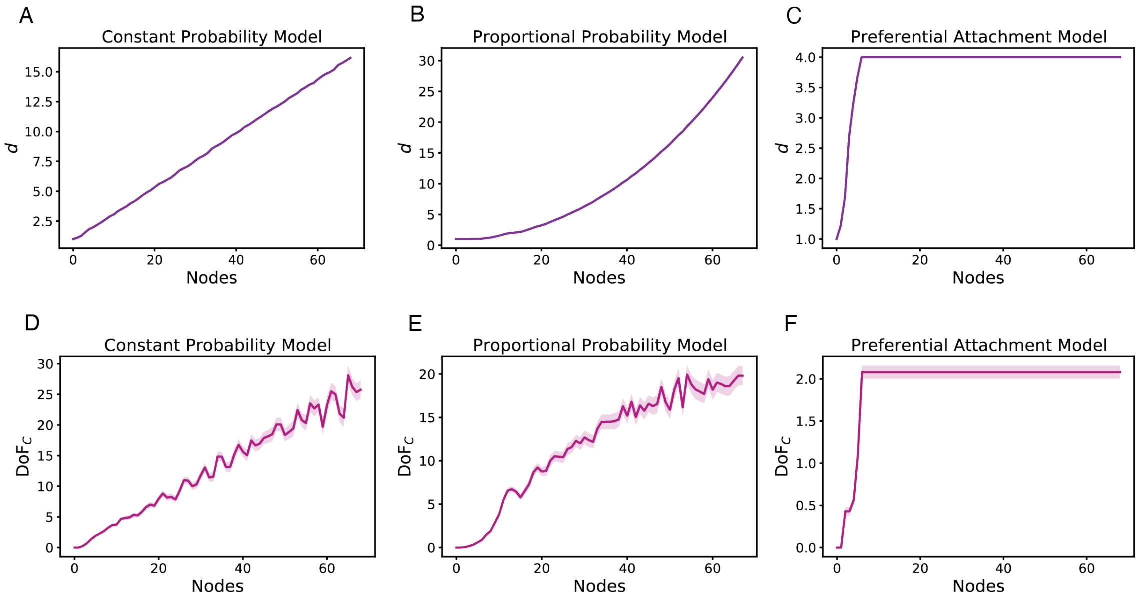


Figure 2: **Embedding dimensionality and conformational flexibility for generative network models.** Embedding dimensionality as a function of network size for the *(A)* constant probability, *(B)* proportional probability, and *(C)* preferential attachment models. Dimensionality increases monotonically for both the constant probability and proportional probability models. However, as opposed to the constant probability model, the rate of increase is non-constant for the proportional probability model. In the preferential attachment model, dimensionality increases to 4 and does not change thereafter. Conformational flexibility as a function of network size for the *(D)* constant probability, *(E)* proportional probability, and *(F)* preferential attachment models. Increases in conformational flexibility are nearly monotonic with network size both for the constant probability and for the proportional probability models. However, both models have functional forms with ragged step-like features. This is likely a consequence of averaging misaligned increments in dimensionality across the ensemble of 100 networks. In the preferential attachment model, the number of conformational degrees of freedom does not change approximately after the addition of node 8 to the growing graphs. Shaded regions represent standard error.

# 4 Results with unnormalized filtration indices

In the main text, for both individual and collective knowledge networks, we normalize the filtration indices to span the range [0, 1], and align values of interest to be defined on the same points before computing the mean for a feature-of-interest across all individuals or topics [23]. For completeness, here we report results with unnormalized values. We note that all empirical feature curves plotted in Fig. 3 through Fig. 5 are significantly different from the feature curves for the corresponding null model data ($p_{perm} < 0.001$).

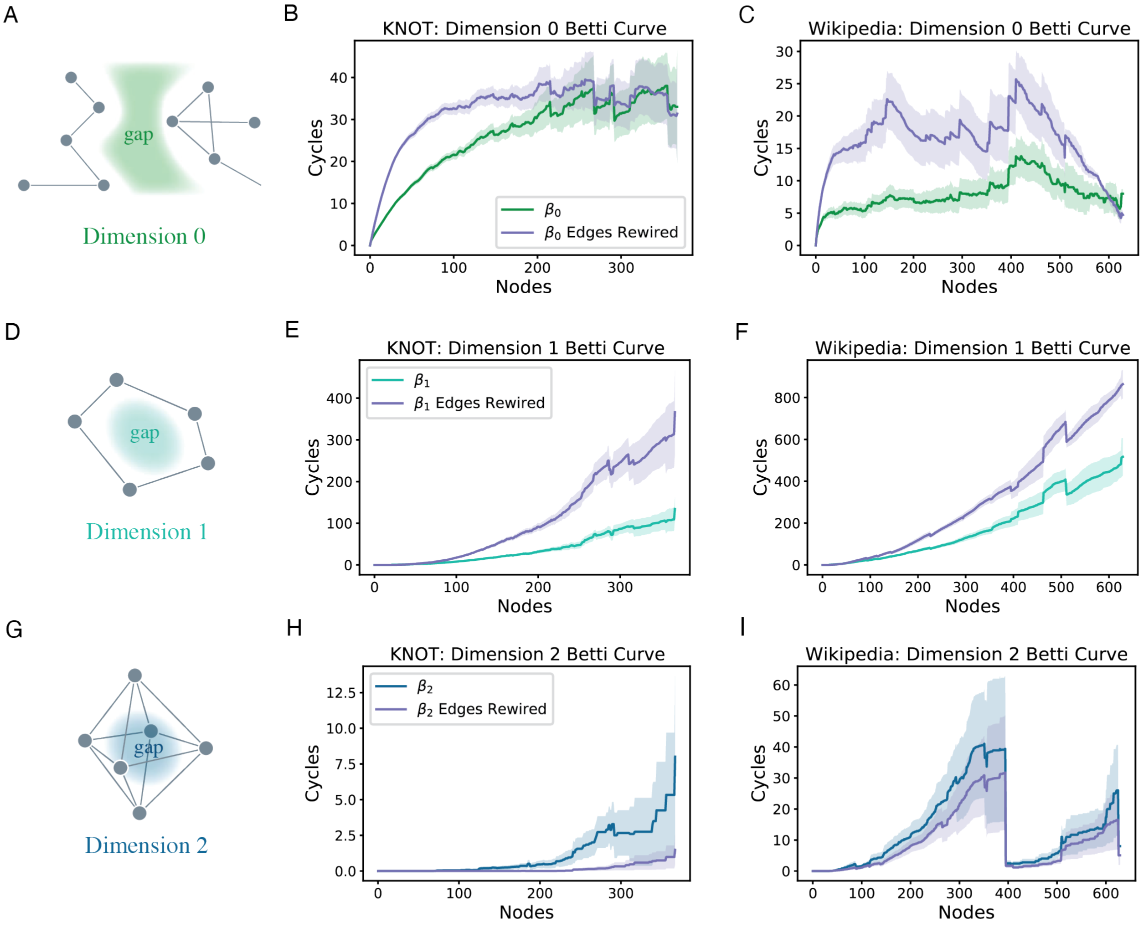


Figure 3: **Probing information gaps as topological cavities in growing knowledge networks.** We operationalize information gaps as topological cavities (also referred to as *cycles*) and track their evolution in growing individual and collective knowledge networks. We plot the number of cycles as a function of time. *(A)* Topological cavities in dimension 0, or 0-cycles, represent disconnected network components. *(B, C)* Individual and collective knowledge networks do not consistently possess fewer disconnected components compared to edge-rewired null model networks. *(D)* In dimension 1, a topological cavity represents an enclosed loop formed by edges. *(E, F)* Growing individual and collective knowledge networks have fewer loops than would be expected to form through random growth. *(G)* A topological cavity in dimension 2 constitutes a void enclosed by 3-cliques, or triangles of interconnected nodes. *(H)* On average, growing individual knowledge networks do not contain 2-dimensional cavities. *(I)* On the other hand, for networks built collectively, overlapping Betti curves for empirical and null model data indicate that the number of 2-dimensional gaps is neither significantly more nor less than would be expected due to random growth. Shaded regions in panels *B,C*, *E,F*, and *H,I* represent standard error. Purple curves denote the average number of cavities in edge-rewired null model networks.

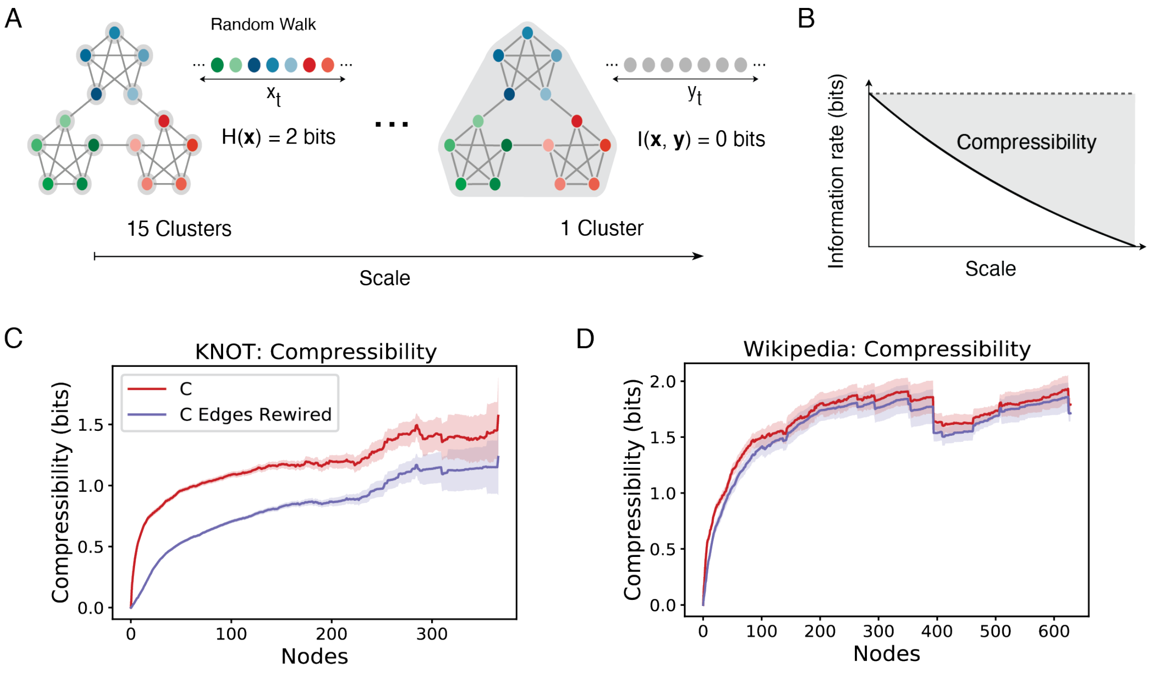


Figure 4: **Measuring compression progress as network compressibility.** *(A)* A random walk $\boldsymbol{x}$ on a network is a sequence of nodes constructed by transitioning from a node $x_t$ to one of its neighbors uniformly at random. Such a sequence generates information at a rate given by its *entropy*, $H(\boldsymbol{x})$. Suppose that we group the network's nodes into clusters. The scale at which the network is viewed can be defined in terms of the number of clusters used. A random walk $\boldsymbol{y}$ on the clustered network is comprised of cluster identities $y_t$ as opposed to node identities $x_t$, where $y_t$ is the cluster that contains node $x_t$. The coarse-grained sequence $\boldsymbol{y}$ has a lower information rate, given by the *mutual information* $I(\boldsymbol{x}, \boldsymbol{y}) = H(\boldsymbol{y}) - H(\boldsymbol{y}|\boldsymbol{x})$, compared to the original unclustered sequence $\boldsymbol{x}$. Mutual information $I(\boldsymbol{x}, \boldsymbol{y})$ is greatest—and equal to the entropy $H(\boldsymbol{x})$—when each node is assigned independently to its own cluster. By contrast, in the limit where the entire network is viewed as one large cluster, mutual information evaluates to 0 bits. *(B)* At every scale of description in between, we can find an optimal clustering that maximally lowers the information rate. Network compressibility is then defined as the average maximal reduction across all scales in the information rate of a random walk. *(C)* Knowledge networks built by individuals are more compressible than corresponding null model networks. *(D)* Knowledge networks built by collectives are neither markedly more nor markedly less compressible than corresponding null model networks. Shaded regions in panels $C$ and $D$ represent standard error. Purple curves denote average compressibility values for edge-rewired null model networks.

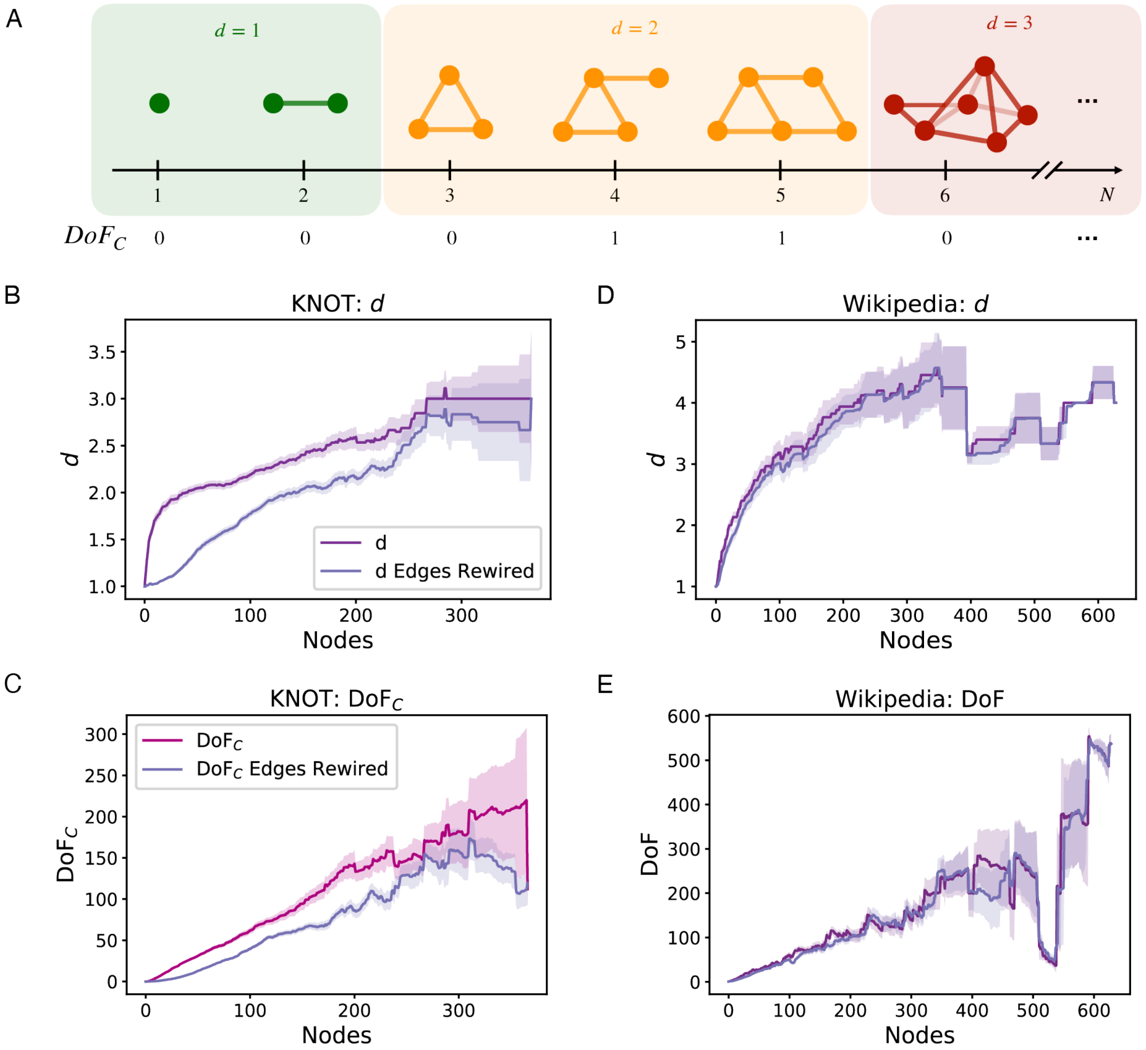


Figure 5: **Conformational change theory of curiosity.** We propose that in the networked space of the mind, while some concepts and their relationships have fixed locations, others move flexibly in a manner that depends upon the context. Such flexibility affords curious learners the ability to rethink and reconfigure what they know in light of new information. We formalize flexibility as the number of conformational degrees of freedom ($DoF_C$). In a network in $d$-dimensional space with $p$ nodes and $q$ edges, $DoF_C = dp - q - d(d+1)/2$. Assuming networks are initially embedded in 1-dimensional space, we compute $DoF_C$ for filtrations of growing knowledge networks. A negative value for the number of conformational degrees of freedom indicates the presence of self-stress that we resolve by incrementing the dimensionality by 1. *(A)* In the example filtration, when nodes 3 and 6 are added, the network becomes over-constrained and develops self-stress. Consequently, the dimensionality first increases from 1 (green) to 2 (orange) and then from 2 (orange) to 3 (red). *(B, C)* Individual knowledge networks require greater dimensionality and possess greater flexibility than related null model networks. *(D, E)* Collective knowledge networks do not exhibit greater dimensionality or conformational flexibility than related null model networks. Shaded regions in panels *B-E* represent standard error. Purple curves denote average values for edge-rewired null model networks.

## 5 References


[1] John O'Keefe and Lynn Nadel. *The Hippocampus as a Cognitive Map*. Oxford: Clarendon Press, 1978. ISBN 0-19-857206-9. URL `http://hdl.handle.net/10150/620894`.

[2] Arne D. Ekstrom, Michael J. Kahana, Jeremy B. Caplan, Tony A. Fields, Eve A. Isham, Ehren L. Newman, and Itzhak Fried. Cellular networks underlying human spatial navigation. *Nature*, 425(6954):184–188, 2003. doi: 10.1038/nature01964. URL `https://doi.org/10.1038/nature01964`.

[3] Torkel Hafting, Marianne Fyhn, Sturla Molden, May-Britt Moser, and Edvard I. Moser. Microstructure of a spatial map in the entorhinal cortex. *Nature*, 436(7052):801–806, 2005. doi: 10.1038/nature03721. URL `https://doi.org/10.1038/nature03721`.

[4] Edvard I. Moser, Emilio Kropff, and May-Britt Moser. Place cells, grid cells, and the brain's spatial representation system. *Annual Review of Neuroscience*, 31(1):69–89, 2008. doi: 10.1146/annurev.neuro.31.061307.090723. URL `https://doi.org/10.1146/annurev.neuro.31.061307.090723`. PMID: 18284371.

[5] Lorelei R. Howard, Amir Homayoun Javadi, Yichao Yu, Ravi D. Mill, Laura C. Morrison, Rebecca Knight, Michelle M. Loftus, Laura Staskute, and Hugo J. Spiers. The hippocampus and entorhinal cortex encode the path and Euclidean distances to goals during navigation. *Current Biology*, 24(12):1331–1340, 2014. ISSN 0960-9822. doi: https://doi.org/10.1016/j.cub.2014.05.001. URL `https://www.sciencedirect.com/science/article/pii/S0960982214005260`.

[6] Martin J. Chadwick, Amy E. J. Jolly, Doran P. Amos, Demis Hassabis, and Hugo J. Spiers. A goal direction signal in the human entorhinal/subicular region. *Current Biology*, 25(1): 87–92, 2015. ISSN 0960-9822. doi: https://doi.org/10.1016/j.cub.2014.11.001. URL `https://www.sciencedirect.com/science/article/pii/S0960982214014274`.

[7] Jacob LS Bellmund, Lorena Deuker, Tobias Navarro Schröder, and Christian F. Doeller. Grid-cell representations in mental simulation. *eLife*, 5:e17089, aug 2016. ISSN 2050-084X. doi: 10.7554/eLife.17089. URL `https://doi.org/10.7554/eLife.17089`.

[8] Daniel Bush, Caswell Barry, Daniel Manson, and Neil Burgess. Using grid cells for navigation. *Neuron*, 87(3):507–520, 2015. ISSN 0896-6273. doi: https://doi.org/10.1016/j.neuron.2015.07.006. URL `https://www.sciencedirect.com/science/article/pii/S0896627315006285`.

[9] Joshua Jacobs, Christoph T. Weidemann, Jonathan F. Miller, Alec Solway, John F. Burke, Xue-Xin Wei, Nanthia Suthana, Michael R. Sperling, Ashwini D. Sharan, Itzhak Fried, and Michael J. Kahana. Direct recordings of grid-like neuronal activity in human spatial navigation. *Nature Neuroscience*, 16(9):1188–1190, 2013. doi: 10.1038/nn.3466. URL `https://doi.org/10.1038/nn.3466`.

[10] Christian F. Doeller, Caswell Barry, and Neil Burgess. Evidence for grid cells in a human memory network. *Nature*, 463(7281):657–661, 2010. doi: 10.1038/nature08704. URL `https://doi.org/10.1038/nature08704`.

[11] R. Quian Quiroga, L. Reddy, G. Kreiman, C. Koch, and I. Fried. Invariant visual representation by single neurons in the human brain. *Nature*, 435(7045):1102–1107, 2005. doi: 10.1038/nature03687. URL `https://doi.org/10.1038/nature03687`.

[12] Marcel Bausch, Johannes Niediek, Thomas P. Reber, Sina Mackay, Jan Boström, Christian E. Elger, and Florian Mormann. Concept neurons in the human medial temporal lobe flexibly represent abstract relations between concepts. *Nature Communications*, 12(1):6164, 2021. doi: 10.1038/s41467-021-26327-3. URL https://doi.org/10.1038/s41467-021-26327-3.

[13] Alexandra O. Constantinescu, Jill X. O'Reilly, and Timothy E. J. Behrens. Organizing conceptual knowledge in humans with a gridlike code. *Science*, 352(6292):1464–1468, 2016. doi: 10.1126/science.aaf0941. URL https://www.science.org/doi/abs/10.1126/science.aaf0941.

[14] Seongmin A. Park, Douglas S. Miller, Hamed Nili, Charan Ranganath, and Erie D. Boorman. Map making: Constructing, combining, and inferring on abstract cognitive maps. *Neuron*, 107 (6):1226–1238.e8, 2021/10/20 2020. doi: 10.1016/j.neuron.2020.06.030. URL https://doi.org/10.1016/j.neuron.2020.06.030.

[15] Seongmin A. Park, Douglas S. Miller, and Erie D. Boorman. Inferences on a multidimensional social hierarchy use a grid-like code. *bioRxiv*, 2021. doi: 10.1101/2020.05.29.124651. URL https://www.biorxiv.org/content/early/2021/01/26/2020.05.29.124651.

[16] Rita Morais Tavares, Avi Mendelsohn, Yael Grossman, Christian Hamilton Williams, Matthew Shapiro, Yaacov Trope, and Daniela Schiller. A map for social navigation in the human brain. *Neuron*, 87(1):231–243, 2015. ISSN 0896-6273. doi: https://doi.org/10.1016/j.neuron.2015.06.011. URL https://www.sciencedirect.com/science/article/pii/S0896627315005243.

[17] Michael Peer, Iva K. Brunec, Nora S. Newcombe, and Russell A. Epstein. Structuring knowledge with cognitive maps and cognitive graphs. *Trends in Cognitive Sciences*, 25 (1):37–54, 2021. ISSN 1364-6613. doi: https://doi.org/10.1016/j.tics.2020.10.004. URL https://www.sciencedirect.com/science/article/pii/S1364661320302503.

[18] William H. Warren. Non-Euclidean navigation. *Journal of Experimental Biology*, 02 2019. ISSN 0022-0949. doi: 10.1242/jeb.187971. URL https://doi.org/10.1242/jeb.187971.

[19] Christoph Zetzsche, Johannes Wolter, Christopher Galbraith, and Kerstin Schill. Representation of space: Image-like or sensorimotor? *Spatial vision*, 22:409–24, 09 2009. doi: 10.1163/156856809789476074.

[20] Thorsten Kluss, William E. Marsh, Christoph Zetzsche, and Kerstin Schill. Representation of impossible worlds in the cognitive map. *Cognitive Processing*, 16(1):271–276, 2015. doi: 10.1007/s10339-015-0705-x. URL https://doi.org/10.1007/s10339-015-0705-x.

[21] William H. Warren, Daniel B. Rothman, Benjamin H. Schnapp, and Jonathan D. Ericson. Wormholes in virtual space: From cognitive maps to cognitive graphs. *Cognition*, 166:152–163, 2017. ISSN 0010-0277. doi: https://doi.org/10.1016/j.cognition.2017.05.020. URL https://www.sciencedirect.com/science/article/pii/S0010027717301373.

[22] Elizabeth R. Chrastil and William H. Warren. From cognitive maps to cognitive graphs. *PLOS ONE*, 9(11):1–8, 11 2014. doi: 10.1371/journal.pone.0112544. URL https://doi.org/10.1371/journal.pone.0112544.

[23] Nicolas H. Christianson, Ann Sizemore Blevins, and Danielle S. Bassett. Architecture and evolution of semantic networks in mathematics texts. *Proceedings of the Royal Society A: Mathe-*

*matical, Physical and Engineering Sciences*, 476(2239):20190741, 2020. doi: 10.1098/rspa.2019.0741. URL https://royalsocietypublishing.org/doi/abs/10.1098/rspa.2019.0741.
